# Supplementary material for: Stochastic Multi-Armed Bandits with Unrestricted Delay Distributions
Source: arXiv:2106.02436 source file (2021-06-04)
Supplement: Supplementary file 1 [file appendix.tex]

\section{Lemma proofs}
\subsection{\Cref{lemma:quantile_bound_chernoff}}
\begin{proof}
    Define $\indicator \{d_s \leq d_i(q)\}$ to be an indicator that on time $s$ that the delay is lower than $d_i(q)$. Note that if arm $i$ was pulled at time $s$, then $\E[\indicator \{d_s \leq d_i(q)\}] \geq q$. Thus,
        \begin{align*}
            \Pr \Big[n_{t +d_i(q)}(i) < \frac{q}{2}  m_t(i) \Big] &\leq \Pr \Big[\sum_{s\leq t: A_s = i} \indicator \{d_s \leq d_i(q)\}  < \frac{q}{2}  m_t(i) \Big]
            \\
            & \leq \Pr \Big[\sum_{s\leq t: A_s = i} \indicator \{d_s \leq d_i(q)\}  < \frac{1}{2}  \sum_{s\leq t: A_s = i} \E[\indicator \{d_s \leq d_i(q)\}] \Big]
            \\
            & \leq \exp \Big(-\frac{1}{8} \sum_{s\leq t: A_s = i} \E[\indicator \{d_s \leq d_i(q)\}] \Big) \leq \exp \Big(-\frac{q}{8} m_t(i) \Big)
        \end{align*}
        The last inequalities derives from Chernoff bound and since $\sum_{s\leq t: A_s = i} \E[\indicator \{d_s \leq d_i(q)\}] \geq q \cdot m_t(i)$.
\end{proof}
\subsection{\Cref{lemma:quantile_bound_hoeffding}}
\begin{proof}
    By definition, $\Pr[d_{s}\leq d_i(q_i)|A_{s}=a] \geq q_i$.
    Hence, by Hoeffding's inequality 
    \[
        \Pr\Big[\frac{1}{m_{t-d_i(q_i)}(i)}\sum_{s=1}^{t-d_i(q_i)}\mathbb{I}\left\{ d_{s}\leq d_i(q_i),A_{s}=a\right\} \leq q_i-\delta\Big]\leq \exp(-2m_{t-d_i(q_i)}(i)\delta^{2})
    \]
    For $\delta=\sqrt{2\log(T)/m_{t-d_i(q_i)}(i)}$ 
    \[
        \Pr\Big[\sum_{s=1}^{t-d_i(q_i)}\indicator\left\{ d_{s}\leq d_i(q_i),A_{s}=a\right\} \leq q_im_{t-d_i(q_i)}(i)-\sqrt{2\log(T)m_{t-d_i(q_i)}(i)}\Big]\leq\frac{1}{T^{4}}
    \]
    Now, note that
    \[
        n_{t}(i)=\sum_{s=1}^{t}\indicator\left\{ s+d_{s}\leq t,A_{s}=a\right\} \geq\sum_{s=1}^{t-d_i(q_i)}\indicator\left\{ d_{s}\leq d_i(q_i),A_{s}=a\right\} 
    \]
    Which implies that with probability of at least $1-T^{-4}$, 
    \[
    n_{t}(i)\geq q_im_{t-d_i(q_i)}(i)-\sqrt{2\log(T) m_{t-d_i(q_i)}(i)}
    \]
\end{proof}

\subsection{\Cref{lemma:reward-dependent-interval-size-bound}}

\section{Theorem proofs}

\subsection{\Cref{thm:SE_arm_quantiles}}
\begin{proof}
    First, since the delays are independent of the rewards, the reward
    estimator is unbiased. By \cref{lemma:estimator_bound}, with high
    probability for any arm $a$ and time $t$ 
    \[
    \abs{\hat{\mu}_{i}-\mu_i}\leq\sqrt{\frac{2\log(T)}{n_{t}(i)}}.
    \]
    This implies that the best arm is never eliminated. The next step
    is to bound from below the number of observations received from each
    arm. Let $\{q_i\}_{a=1}^{K}:q_i\in(0,1]$ be a set of probabilities
    of our choice and let $d_{max}(i)=\max\{d_i(q_i),d_{i^{*}}(q_{i^{*}})\}$.
    Consider a failure event for all arms, 
    \[
    \mathcal{F}=\left\{ \exists a,\;m_{t}(i)\geq\frac{32\log(T)}{q_i}~:~n_{t+d_{max}({i})+K}(i)<\frac{q_i}{2}m_{t}(i)\right\} .
    \]
    With a union bound and \cref{lemma:quantile_bound_chernoff} we bound the
    probability of $\mathcal{F}$, a similar argument bounds $\mathcal{F_{*}}$.
    \begin{align*}
    \Pr[\mathcal{F}] & =\Pr\Big[\exists i\neq i^{*},\;m_{t}(i)\geq\frac{32\log(T)}{q_i}~:~n_{t+d_{max}(i)+K}(i)<\frac{q_i}{2}m_{t}(i)\Big]\\
     & \tag{union bound}\leq\sum_{i\neq i^{*}}\sum_{t:m_{t}(i)\geq32\log(T)/q_i}\Pr\Big[n_{t+d_{max}(i)+K}(i)<\frac{q_i}{2}m_{t}(i)\Big]\\
     & \leq\sum_{i\neq i^{*}}\sum_{t:m_{t}(i)\geq32\log(T)/q_i}\Pr\Big[n_{t+d_i(q_i)}(i)<\frac{q_i}{2}m_{t}(i)\Big]\\
     & \tag{\cref{lemma:quantile_bound_chernoff}}\leq\sum_{i\neq i^{*}}\sum_{t:m_{t}(i)\geq32\log(T)/q_i}\exp\Big(-\frac{q_i}{8}m_{t}(i)\Big)\\
     & \leq T\cdot K\exp\Big(-\frac{q_i}{8}\frac{32\log(T)}{q_i}\Big)\leq\frac{1}{T^{2}}.
    \end{align*}
    The probability of $\mathcal{F}$ is negligible, thus we'll assume
    this event does not occur. Let $t_i$ be the last time arm $a$
    was pulled. Since $i^{*}$ is never eliminated under the good event,
    \[
        UCB_{t_i}(i)\geq LCB_{t_i}({i^{*}})
    \]
    Denote $\lambda_{t}(i)=\sqrt{\frac{2\log(T)}{n_{t}(i)}}$, the above
    implies that 
    \[
        \mu_i+2\lambda_{t_i}(i)\geq\mu_{i^{*}}-2\lambda_{t_i}({i^{*}})
    \]
    Since $\mathcal{F}$ does not occur, $n_{t_i}(i)>(q_i/2)m_{t_i-d_{max}(i)-K}(i),n_{t_i}({i^{*}})\geq(q_{i^{*}}/2)m_{t_i-d_{max}(i)-K}(i)$.
    So we get that, 
    \begin{align*}
        \Delta_i & \leq 2\sqrt{\frac{2\log(T)}{q_i m_{t_i-d_{max}(i)-K}(i)}}+2\sqrt{\frac{2\log(T)}{q_{i^{*}}m_{t_i-d_{max}(i)-K}(i)}}
        \\
        & \leq 8\sqrt{\frac{\log(T)}{q_i m_{t_i-d_{max}(i)-K}(i)}+\frac{\log(T)}{q_{i^{*}}m_{t_i-d_{max}(i)-K}(i)}}
    \end{align*}
    where the last inequality uses $\sqrt{a}+\sqrt{b}\leq2\sqrt{a+b}$. Now, this implies that,
    $$
        m_{t_i-d_{max}(i)-K}(i) \leq 64\frac{\log(T)}{(\Delta_i)^{2}}\left(\frac{1}{q_i}+\frac{1}{q_{i^{*}}}\right).
    $$
    The regret of arm $i$ is therefore,
    \begin{align*}
    m_{t_i}(i)\Delta_i & \leq (m_{t_i-d_{max}(i)-K}(i)+m_{t_i}(i)-m_{t_i-d_{max}(i)-K}(i))\Delta_i\\
     & \leq 64\frac{\log(T)}{\Delta_i}\left(\frac{1}{q_i}+\frac{1}{q_{i^{*}}}\right)+(m_{t_i}(i)-m_{t_i-d_{max}(i)-K}(i))\Delta_i
    \end{align*}
    Let $\sigma\in S_{K}$ such that $\sigma(i)$ represent order in which
    $a$ was eliminated (e.g. if $\sigma(i)=1$ then $i$ is the first
    arm to be eliminated), where we break ties arbitrarily. Since
    we round-robin over the remaining arms,
    \[
    m_{t_i}(i)-m_{t_i-d_{max}(i)-K}(i)\leq\frac{d_{max}(i)+K}{K-\sigma(i)}
    \]
    So the total regret can be bounded as
    \begin{align*}
    \mathcal{R}_{T} & \leq 64\sum_{i\ne i^{*}}\frac{\log(T)}{\Delta_i}\left(\frac{1}{q_i}+\frac{1}{q_{i^{*}}}\right)+\sum_{i\ne i^{*}}\mathbb{E}\left[\frac{d_{max}(i)}{K-\sigma(i)}\Delta_i+\frac{K}{K-\sigma(i)}\right]\\
     & \leq64\sum_{i\ne i^{*}}\frac{\log(T)}{\Delta_i}\left(\frac{1}{q_i}+\frac{1}{q_{i^{*}}}\right)+\max_{\sigma\in S_{K}}\sum_{i\ne i^{*}}\frac{d_i(q_i)}{K-\sigma(i)}\Delta_i+d_{i^*}(q_{i^*})\log(K)+K\log(K)
    \end{align*}
    
    Since the above holds for any choice of vector $q=(q^1,...,q^K)$, we can choose the vector that minimizes the regret.
\end{proof}
\subsection{\Cref{thm:se_reward_indep_phased}}
\begin{proof}
    First, since the delays are independent of the rewards, the reward estimator is unbiased. From \cref{lemma:estimator_bound}, with high probability for any arm $i$ and time $t$
    \[
        \abs{\hat{\mu}_i - \mu_i} \leq \sqrt{\frac{2\log(T)}{n_t(i)}}.
    \]
    This implies that the best arm is never eliminated. The next step is to bound from below the number of observations received from each arm. Let $\vec{q} \in(0,1]^K$ be a probability of a quantile for each arm and let $d_{max} = \max_{i \neq i^*}d_i(q_i)$. Consider the following failure event,
    \[
    \mathcal{F}=\left\{ \exists a \in [K], \; m_t(i) \geq \frac{32\log(T)}{q_i} ~:~ n_{t+d_{max}}(i)<\frac{q_i}{2} m_t(i)\right\} .
    \]
    With a union bound and \cref{lemma:quantile_bound_chernoff} we have, 
    \begin{align*}
        \Pr [ \mathcal{F}] &= \Pr \Big[\exists a \in [K], \; m_t(i) \geq \frac{32\log(T)}{q_i} ~:~ n_{t+d_{max}}(i)<\frac{q_i}{2} m_t(i) \Big] 
        \\
        & \tag{union bound} \leq \sum_i  \sum_{t: m_t(i) \geq 32\log(T)/q_i} \Pr \Big[n_{t+d_{max}}(i)<\frac{q_i}{2} m_t(i) \Big]
        \\
        & \leq \sum_i  \sum_{t: m_t(i) \geq 32\log(T)/q_i} \Pr \Big[n_{t+d_{i}(q_i)}(i) < \frac{q_i}{2} m_t(i) \Big]
        \\
        & \tag{\cref{lemma:quantile_bound_chernoff}} \leq \sum_i \sum_{t: m_t(i) \geq 32\log(T)/q_i}  \exp \Big(-\frac{q_i}{8} m_t(i) \Big)
        \\
        &  \leq T \cdot K \exp \Big(-\frac{q_i}{8} \frac{32\log(T)}{q_i} \Big) \leq \frac{1}{T^2}.
    \end{align*}
    The probability of $\mathcal{F}$ is negligible, thus we'll assume this event does not occur. For $i \in [K]$, define
    $$
        t_{\ell}(i) = \tau_i\big(32\log(T)/(q_i\epsilon_{\ell}^2)\big)
    $$
    The time we pulled arm $i$ exactly $32\log(T)/(q_i\epsilon_{\ell}^2)$ times. If arm $i$ was eliminated before that, then $t_{\ell}(i)$ is defined as the total amount of pulls of arm $i$. Since $\mathcal{F}$ does not occur, 
    $$
        n_{t_{\ell}(i) + d_{max}}(i) \geq (q_i/2)m_{t_{\ell}(i)}(i) = 16\log(T)/\epsilon_{\ell}^2.
    $$ 
    Suppose arm $i$ was eliminated at the end of phase $\ell+1$. Then, by time $t_{\ell+1}(i) + d_{max}$ we stopped pulling arm $i$ at phase $\ell+1$. Moreover, as arm $i$ was not eliminated at the end of phase $\ell$,
    \[
        UCB_{t_{\ell}}(i) \geq LCB_{t_{\ell}}(i^*).
    \]
    Where $t_{\ell}$ is the time phase $\ell$ ended. This implies that,
    \[
        \mu_{i^{*}}-\mu_{i}=\Delta_{i}\leq 2\sqrt{\frac{2\log(T)}{n_{t_{\ell}}(i)}} + 2\sqrt{\frac{2\log(T)}{n_{t_{\ell}}(i^*)}}  \leq 4\sqrt{\frac{2\log(T)}{16\log(T)/\epsilon_{\ell}^2}} \leq 2\epsilon_{\ell} = 4\epsilon_{\ell+1}.
    \]
    Let $S_{\ell}$ be the set of arms that were eliminated at the end of phase $\ell+1$. The total regret for $S_{\ell}$ is:
    \begin{align*}
        \sum_{i \in S_{\ell}} m_{t_{\ell+1}(i)+d_{max}}(i)\Delta_i & =\sum_{i \in S_{\ell}} \big(m_{t_{\ell+1}(i)+d_{max}}(i)-m_{t_{\ell+1}(i)}(i)\big)\Delta_i + \sum_{i \in S_{\ell}}  m_{t_{\ell+1}(i)}(i)\Delta_i
        \\
         & \leq \sum_{i \in S_{\ell}}  2\epsilon_{\ell}\big(m_{t_{\ell+1}(i)+d_{max}}(i)-m_{t_{\ell+1}(i)}(i)\big) + \sum_{i \in S_{\ell}} \frac{32\log(T)}{q_i\epsilon_{\ell+1}^{2}}\Delta_i
         \\
         & \leq \epsilon_{\ell-1} \sum_{i \in S_{\ell}} \big(m_{t_{\ell+1}(i)+d_{max}}(i)-m_{t_{\ell+1}(i)}(i)\big) + \sum_{i \in S_{\ell}} \frac{512\log(T)}{q_i\Delta_i}
    \end{align*}
    For arm $i \in S_{\ell}$, let $k_{\ell+1}(i)$ be the number of active arms we need to pull at time $t_{\ell+1}(i)+d_{max}$ . Then, since we round robin over the arms, between time $t_{\ell+1}(i)+d_{max}$ and time $t_{\ell+1}(i)$ we pulled arm $i$ at most $d_{max}/k_{\ell+1}(i)$. Hence,
    $$
        \sum_{i \in S_{\ell}}  \big(m_{t_{\ell+1}(i)+d_{max}}(i)-m_{t_{\ell+1}(i)}(i)\big) \leq \sum_{i \in S_{\ell}} \frac{d_{max}}{k_{\ell+1}(i)} \leq \sum_{i=1}^K \frac{d_{max}}{K-(i-1)} \leq \log(K) d_{max}
    $$
    
   Summing over all phases, would give us a total regret of, 
    \[
        \mathcal{R_{T}} \leq \sum_{\ell=1}^{\infty} \Big(\epsilon_{\ell-1} \log(K) d_{max} + \sum_{i \in S_{\ell}} \frac{512\log(T)}{q_i\Delta_i}\Big) \leq \sum_{i \neq i^*}\Big(\frac{512\log(T)}{q_i\Delta_i}\Big)+2\log(K)\max_{i \neq i^*}d_i(q_i).
    \]
    The above is true for any choice of $q \in (0,1]^K$, thus we choose the optimal $q$ to obtain the statement of the theorem.
\end{proof}
\subsection{\Cref{thm:se_reward_dep}}
\begin{proof}
    Let some vector $q \in (0,1]^K$ (which will be determined later). We assume throughout
    the proof that $\lnot F\left(q\right)$ occur and that, 
    \[
        \forall a,t:\left|\tilde{\mu}_{t}(i)-\mu_i\right|\leq\sqrt{\frac{2\log T}{m_{t}(i)}}
    \]
    As mentioned each of the events occur with probability of at least
    $1-T^{-2}$ and so using the union bound both event occur with probability
    of at least $1-2T^{-2}$.
    
    Note that, under the good event, the best arm is never eliminated,
    since otherwise: 
    \[
        \mu_{i^{*}} \leq \tilde{\mu}_t({i^{*}})+\sqrt{\frac{2\log T}{m_{t}(i^{*})}}\leq\hat{\mu}^{+}_t({i^*})+\sqrt{\frac{2\log T}{m_{t}(i^{*})}}=UCB_{t}(i^{*})<LCB_{t}(i)=\hat{\mu}_{t}^{-}(i)-\sqrt{\frac{2\log T}{m_{t}(i)}}\leq\tilde{\mu}_t({i})-\sqrt{\frac{2\log T}{m_{t}(i)}}\leq\mu_i
    \]
    Which contradicts $\mu_{i^{*}}$ optimality.
    
    Under the good event, we have that 
    \begin{align*}
         & UCB_{t}(i)=\hat{\mu}_{t}^{+}(i)+\sqrt{\frac{2\log T}{m_{t}(i)}}\\
         & \leq\tilde{\mu}_t({i})+\frac{m_{t}(i)-m_{t-d_i(q_i)}(i)}{m_{t}(i)}+1-q_i+2\sqrt{\frac{2\log T}{m_{t}(i)}}\\
         & \leq\mu_i+\frac{m_{t}(i)-m_{t-d_i(q_i)}(i)}{m_{t}(i)}+1-q_i+3\sqrt{\frac{2\log T}{m_{t}(i)}},
    \end{align*}
    Where the first inequality holds from \cref{lemma:reward-dependent-interval-size-bound}. In a similar
    way, 
    \begin{align*}
         & LCB_{t}(i^{*})=\hat{\mu}^{-}_t(i^{*})-\sqrt{\frac{2\log T}{m_{t}(i^{*})}}
         \\
         & \geq\tilde{\mu}_t({i^{*}}) - \frac{m_{t}(i^{*}) - m_{t-d_{i^*}(q_{i^{*}})}({i^{*}})}{m_{t}(i^{*})}-(1-q_{i^*})-2\sqrt{\frac{2\log T}{m_{t}(i^{*})}}
         \\
         & \geq\mu_{i^{*}}-\frac{m_{t}(i^{*})-m_{t-d_{i^*}(q_{i^{*}})}({i^{*}})}{m_{t}(i^{*})}-(1-q_{i^*})-3\sqrt{\frac{2\log T}{m_{t}(i^{*})}}
    \end{align*}
    Let $t_i$ be the last round that $i$ was chosen, then $LCB_{t_i}({i^{*}})\leq UCB_{t_i}(i)$
    (since $i$ is not yet eliminated at time $t_i$). 
    \[
    \Delta_i-(1-q_i)-(1-q_{i^{*}})\leq\frac{m_{t_i}(i)-m_{t_i-d_i(q_i)}(i)}{m_{t_i}(i)}+\frac{m_{t_i}({i^{*}})-m_{t_i-d({i^{*}})(q_{i^{*}})}({i^{*}})}{m_{t_i}({i^{*}})}+3\sqrt{\frac{2\log T}{m_{t_i}(i)}}+3\sqrt{\frac{2\log T}{m_{t_i}({i^{*}})}}
    \]
    Set $q_{i^{*}}=q_i=1-\Delta_i/4$. Define the following:
    \begin{align*}
        d_{max} & =\max_{i\ne i^{*}}d_i(1-\Delta_i/4)\\
        d_{max}^* & =\max_{i\ne i^{*}}d_{i^*}(1-\Delta_i/4)=d_{i^*}(1-\min_{i\ne i^{*}}\Delta_i/4)
    \end{align*}
    Recall that $\left|m_{t}(i)-m_{t}(i^{*})\right|\leq1$
    for any $t\leq t_i$. Hence, 
    \[
        \Delta_i\leq2\frac{m_{t_i}(i)-m_{t_i-d_{max}}(i)+m_{t_i}(i)-m_{t_i-d_{max}^*}(i)+2}{m_{t_i}(i)}+12\sqrt{\frac{2\log T}{m_{t_i}(i)}}
    \]
    If the first term above dominates
    then,
    \[
        m_{t}(i)\Delta_i\leq4\left(m_{t_i}(i)-m_{t_i-d_{max}}(i)+m_{t_i}(i)-m_{t_i-d_{max}^*}(i)+2\right)
    \]
    If the second term dominates
    then, 
    \[
        m_{t}(i)\Delta_i\leq \frac{1152\log T}{\Delta_i}\
    \]
    Overall we get that the total regret from arm $i$ is at most 
    \[
        m_{t_i}(i)\Delta_i\leq \frac{1152\log T}{\Delta_i}+4(m_{t_i}(i)-m_{t_i-d_{max}}(i)+m_{t_i}(i)-m_{t_i-d_{max}^*}(i)) + 8
    \]
    Denote by $k_i$ the number of arms that remained at time $t_i$.
    Then for any $d$ 
    \[
        m_{t_i}(i)-m_{t_i-d}(i)\leq\frac{d}{k_i}
    \]
    Hence, the total regret for arm $i$ is at most 
    \[
        \frac{1152\log T}{\Delta_i}+\frac{4(d_{max}+d_{max}^{*})}{k_i} + 8
    \]
    Without lose of generality, $k_i=i$. This implies that the above
    is at most
    \begin{align*}
         & \sum_{i\ne i^{*}}\frac{1152\log T}{\Delta_i}+4\left(d_{max}+d_{max}^{*}\right)\sum_{i=1}^{K-1}\frac{1}{i} + 8K
         \\
         & \leq \sum_{i\ne i^{*}}\frac{1152\log T}{\Delta_i}+4\log\left(K\right)\left(\max_{i\ne i^{*}}d_i(1-\Delta_i/4)+d_{i^*}(1-\min_{i\ne i^{*}}\Delta_i/4)\right) + 8K
    \end{align*}
\end{proof}

\section{Reward-independent additional theorems}
\subsection{Fixed delays theorem}
\label{appendix:fixed_delay}
TODO
\subsection{Proof of \Cref{thm:SE_single_quantile}}

Fix $q\in(0,1]$, let $\tau(r)$ be the time we pulled all the active arms exactly $r$ times and define $t_{\ell}=\tau\left(\frac{32\log T}{q\epsilon_{\ell}^{2}}\right)$.
We define the next two faliure events:
\[
F_{1} = 
\left\{ \exists t,i: \abs{\hat{\mu}_{t}(i) - \mu_{t}(i)}>\sqrt{\frac{2\log(T)}{n_{t}(i)}} \right\} 
\]
\[
F_{2} = 
\left\{ \exists t>t_{0}\exists i: n_{t+\max_{i}d_{i}(q)+K}(i) < \frac{1}{2}qm_{t}(i) \right\} ,
\]
and the clean event $G=\lnot F_{1} \cap \lnot F_{2}$. Using \cref{lemma:estimator_bound}, \cref{lemma:quantile_bound_chernoff} and union bound, $P(G)\geq1-2T^{-2}$. Note that under the event $G$, $i^{*}$ is never eliminated. Hence, if $i$ was \textit{not} eliminated by time $t_{\ell}+\max_{i}d_{i}(q)+K$, then 
\[
UCB_{t_{\ell} + \max_{i}d_{i}(q)+K}(i)\
\geq 
LCB_{t_{\ell} + \max_{i}d_{i}(q)+K}(i^{*})\
\]
The above implies that 
\[
\mu_{i^{*}} - \mu_{i} 
\leq 
2\sqrt{\frac{2\log(T)}{n_{t_{\ell} + \max_{i}d_{i}(q)+K}(i)}} + 2\sqrt{\frac{2\log(T)}{n_{t_{\ell} + \max_{i}d_{i}(q)+K}(i^{*})}}
\]
Under the event $G$, 
\[
n_{t_{\ell} + \max_{i}d_{i}(q)+K}(i), n_{t_{\ell} + \max_{i}d_{i}(q) + K}(i^{*})
\geq
16\log(T)/\epsilon_{\ell}^{2}
\]
We get that, if $i$ was \textit{not} eliminated by time $t_{\ell} + \max_{i}d_{i}(q) + K$,
then
\begin{equation}    \label{eq:fixed-q-delta-bound}
\Delta_{i} 
= \mu_{i^{*}} - \mu_{i} 
\leq 
2\epsilon_{\ell} 
= 4\epsilon_{\ell+1}
\end{equation}
Let $S_{\ell}$ be the set of arms that were \textit{not} eliminated
by time $t_{\ell}+\max_{i}d_{i}(q)+K$, but were eliminated by time
$t_{\ell+1}+\max_{i}d_{i}(q)+K$. If $t_{\ell+1}+\max_{i}d_{i}(q)+K>T$,
then $S_{\ell}$ contains all the remaining arms. The total regret
from arms in $S_{\ell}$ is 
\begin{align*}
& \sum_{i\in S_{\ell}}m_{t_{\ell + 1} + \max_{i}d_{i}(q) + K}(i)\Delta_{i} \\
& =
\sum_{i\in S_{\ell}} \big(m_{t_{\ell + 1} + \max_{i}d_{i}(q) + K}(i)-m_{t_{\ell + 1}}(i)\big)\Delta_{i} + \sum_{i\in S_{\ell}}m_{t_{\ell + 1}}(i)\Delta_{i}\\
& \leq
4\epsilon_{\ell}\sum_{i\in S_{\ell}}\big(m_{t_{\ell + 1} + \max_{i}d_{i}(q) + K}(i)-m_{t_{\ell + 1}}(i)\big) + \sum_{i\in S_{\ell}}\frac{32\log(T)}{q\epsilon_{\ell + 1}^{2}}\Delta_{i}\\
\tag{by \ref{eq:fixed-q-delta-bound}}
& \leq
4\epsilon_{\ell}\sum_{i}\big(m_{t_{\ell + 1} + \max_{i}d_{i}(q) + K}(i)-m_{t_{\ell + 1}}(i)\big) + \sum_{i\in S_{\ell}}\frac{512\log(T)}{q\Delta_{i}}\\
& =
4\epsilon_{\ell}(t_{\ell + 1}-t_{\ell + 1} + \max_{i}d_{i}(q) + K) + \sum_{i\in S_{\ell}}\frac{512\log(T)}{q\Delta_{i}}\\
& =
4\epsilon_{\ell}(\max_{i}d_{i}(q) + K) + \sum_{i\in S_{\ell}}\frac{512\log(T)}{q\Delta_{i}}
\end{align*}
Summing over all $\ell$, taking into account the arms that where
eliminated before time $t_{0}+\max_{i}d_{i}(q)+K$ and the regret
given $\lnot G$,
\[
\mathcal{R}_{T}
\leq \sum_{i} \frac{544\log(T)}{q\Delta_{i}} + 10\max_{i}d_{i}(q) + 10K + \frac{2}{T}
\]
The above is true for any non-zero choice of $q$, thus we choose
the optimal $q$ to obtain the statement of the theorem.

\section{Omitted proofs}
\subsection{Proof of \Cref{thm:SE_single_quantile}}

Fix $q\in(0,1]$, let $\tau(r)$ be the time we pulled all the active arms exactly $r$ times and define $t_{\ell}=\tau\left(\frac{32\log T}{q\epsilon_{\ell}^{2}}\right)$.
We define the next two faliure events:
\[
F_{1} = 
\left\{ \exists t,i: \abs{\hat{\mu}_{t}(i) - \mu_{t}(i)}>\sqrt{\frac{2\log(T)}{n_{t}(i)}} \right\} 
\]
\[
F_{2} = 
\left\{ \exists t>t_{0}\exists i: n_{t+\max_{i}d_{i}(q)+K}(i) < \frac{1}{2}qm_{t}(i) \right\} ,
\]
and the clean event $G=\lnot F_{1} \cap \lnot F_{2}$. Using \cref{lemma:estimator_bound}, \cref{lemma:quantile_bound_chernoff} and union bound, $P(G)\geq1-2T^{-2}$. Note that under the event $G$, $i^{*}$ is never eliminated. Hence, if $i$ was \textit{not} eliminated by time $t_{\ell}+\max_{i}d_{i}(q)+K$, then 
\[
UCB_{t_{\ell} + \max_{i}d_{i}(q)+K}(i)\
\geq 
LCB_{t_{\ell} + \max_{i}d_{i}(q)+K}(i^{*})\
\]
The above implies that 
\[
\mu_{i^{*}} - \mu_{i} 
\leq 
2\sqrt{\frac{2\log(T)}{n_{t_{\ell} + \max_{i}d_{i}(q)+K}(i)}} + 2\sqrt{\frac{2\log(T)}{n_{t_{\ell} + \max_{i}d_{i}(q)+K}(i^{*})}}
\]
Under the event $G$, 
\[
n_{t_{\ell} + \max_{i}d_{i}(q)+K}(i), n_{t_{\ell} + \max_{i}d_{i}(q) + K}(i^{*})
\geq
16\log(T)/\epsilon_{\ell}^{2}
\]
We get that, if $i$ was \textit{not} eliminated by time $t_{\ell} + \max_{i}d_{i}(q) + K$,
then
\begin{equation}    \label{eq:fixed-q-delta-bound}
\Delta_{i} 
= \mu_{i^{*}} - \mu_{i} 
\leq 
2\epsilon_{\ell} 
= 4\epsilon_{\ell+1}
\end{equation}
Let $S_{\ell}$ be the set of arms that were \textit{not} eliminated
by time $t_{\ell}+\max_{i}d_{i}(q)+K$, but were eliminated by time
$t_{\ell+1}+\max_{i}d_{i}(q)+K$. If $t_{\ell+1}+\max_{i}d_{i}(q)+K>T$,
then $S_{\ell}$ contains all the remaining arms. The total regret
from arms in $S_{\ell}$ is 
\begin{align*}
& \sum_{i\in S_{\ell}}m_{t_{\ell + 1} + \max_{i}d_{i}(q) + K}(i)\Delta_{i} \\
& =
\sum_{i\in S_{\ell}} \big(m_{t_{\ell + 1} + \max_{i}d_{i}(q) + K}(i)-m_{t_{\ell + 1}}(i)\big)\Delta_{i} + \sum_{i\in S_{\ell}}m_{t_{\ell + 1}}(i)\Delta_{i}\\
& \leq
4\epsilon_{\ell}\sum_{i\in S_{\ell}}\big(m_{t_{\ell + 1} + \max_{i}d_{i}(q) + K}(i)-m_{t_{\ell + 1}}(i)\big) + \sum_{i\in S_{\ell}}\frac{32\log(T)}{q\epsilon_{\ell + 1}^{2}}\Delta_{i}\\
\tag{by \ref{eq:fixed-q-delta-bound}}
& \leq
4\epsilon_{\ell}\sum_{i}\big(m_{t_{\ell + 1} + \max_{i}d_{i}(q) + K}(i)-m_{t_{\ell + 1}}(i)\big) + \sum_{i\in S_{\ell}}\frac{512\log(T)}{q\Delta_{i}}\\
& =
4\epsilon_{\ell}(t_{\ell + 1}-t_{\ell + 1} + \max_{i}d_{i}(q) + K) + \sum_{i\in S_{\ell}}\frac{512\log(T)}{q\Delta_{i}}\\
& =
4\epsilon_{\ell}(\max_{i}d_{i}(q) + K) + \sum_{i\in S_{\ell}}\frac{512\log(T)}{q\Delta_{i}}
\end{align*}
Summing over all $\ell$, taking into account the arms that where
eliminated before time $t_{0}+\max_{i}d_{i}(q)+K$ and the regret
given $\lnot G$,
\[
\mathcal{R}_{T}
\leq \sum_{i} \frac{544\log(T)}{q\Delta_{i}} + 10\max_{i}d_{i}(q) + 10K + \frac{2}{T}
\]
The above is true for any non-zero choice of $q$, thus we choose
the optimal $q$ to obtain the statement of the theorem.

\section{Refined analysis of SE}
\subsection{Analysis via Exponentially Decaying Sets}
Define $S_i = \{a : \epsilon_{i+1} < \Delta^a \leq \epsilon_{i}\}$, where $\epsilon_{i} = 2^{-i}$. Let $\sigma(i) = i$ such that $a \in S_i$. Note that $\sigma$ is not defined for the best arm. Separating the arms into exponentially decaying sets gives us a more refined bound on the regret in comparison to \cref{thm:se_reward_indep}. Instead of choosing a single quantile $q$ for all arms, we can choose one per $S_i$. 
\begin{theorem}
    \label{thm:se_reward_indep_refined}
    For reward-independent delay distributions $\{D^a\}_{a=1}^K$, the expected pseudo-regret of \cref{alg:non-phased-SE} is bounded by
    \begin{align*}
        \mathcal{R}_{T} & \leq \min_{\{q(i)\}_{i=1}^{\infty}:~q(i) \in (0,1]} \sum_{a \neq a^*}\Big(\frac{512\log\left(T\right)}{q({\sigma(i)})\Delta_i}\Big)+2\max_{a \neq a^*}d^{\max\{a, a^*\}}\big(q({\sigma(i)})\big) + 2K
    \end{align*}
\end{theorem}

\begin{proof}
    First, since the delays are independent of the rewards, the reward estimator is unbiased. By \cref{lemma:estimator_bound}, with high probability for any arm $a$ and time $t$
    \[
        \abs{\hat{\mu}^a - \mu^a} \leq \sqrt{\frac{2\log(T)}{n_t^a}}.
    \]
    This implies that the best arm is never eliminated. The next step is to bound from below the number of observations received from each arm. Let $\{q(i)\}_{i=1}^{\infty}: q(i) \in (0,1]$ be a set of probabilities of our choice and let $d_{max} = \max_{i}d^{\max\{a, a^*\}}(q(\sigma(i)))$. Consider a failure event for all non-best arms,
    \[
        \mathcal{F}=\left\{ \exists a \neq a^*, \; m_t^a \geq \frac{32\log(T)}{q({\sigma(i)})} ~:~ n_{t+d_{max}+K}^a<\frac{q({\sigma(i)})}{2} m_t^a\right\} .
    \]
    Similarly, we define a failure event for the best arm,
    \[
        \mathcal{F_{*}}=\left\{ \exists a \neq a^*, \; m_t({i^*}) \geq \frac{32\log(T)}{q({\sigma(i)})} ~:~ n_{t+d_{max}+K}({i^*})<\frac{q({\sigma(i)})}{2} m_t({i^*})\right\} .
    \]
    With a union bound and \cref{lemma:quantile_bound_chernoff} we bound the probability of $\mathcal{F}$, a similar argument bounds $\mathcal{F_{*}}$.
    \begin{align*}
        \Pr [ \mathcal{F}] &= \Pr \Big[\exists a \neq a^*, \; m_t^a \geq \frac{32\log(T)}{q({\sigma(i)})} ~:~ n_{t+d_{max}+K}^a<\frac{q({\sigma(i)})}{2} m_t^a \Big] 
        \\
        & \tag{union bound} \leq \sum_{a \neq a^*} \sum_{t: m_t^a \geq 32\log(T)/q({\sigma(i)})}  \Pr \Big[n_{t+d_{max}+K}^a<\frac{q({\sigma(i)})}{2} m_t^a \Big]
        \\
        & \leq \sum_{a \neq a^*} \sum_{t: m_t^a \geq 32\log(T)/q({\sigma(i)})}  \Pr \Big[n_{t+d_i(q({\sigma(i)}))}^a < \frac{q({\sigma(i)})}{2} m_t^a \Big]
        \\
        & \tag{\cref{lemma:quantile_bound_chernoff}} \leq \sum_{a \neq a^*} \sum_{t: m_t^a \geq 32\log(T)/q({\sigma(i)})} \exp \Big(-\frac{q({\sigma(i)})}{8} m_t^a \Big)
        \\
        &  \leq T \cdot K \exp \Big(-\frac{q({\sigma(i)})}{8} \frac{32\log(T)}{q({\sigma(i)})} \Big) \leq \frac{1}{T^2}.
    \end{align*}
    The probability of $\mathcal{F}$ is negligible, thus we'll assume this event does not occur. 
    Let $t_{i}=\tau\left(\frac{32 \log (T)}{q(i) \epsilon_i^2}\right)$. By time $t_{i+2}+d_{max}+K$ all arms from $S_i$ were eliminated, as otherwise
    \[
        UCB^{a}_{t_{i+2}+d_{max}+K} \geq LCB({i^{*}})_{t_{i+2}+d_{max}+K}
    \]
    Denote $\lambda^{a}_t=\sqrt{\frac{2\log(T)}{n^{a}_{t}}}$, the above
    implies that 
    \[
    \mu_i+2\lambda^{a}_{t_{i+2}+d_{max}+K}\geq\mu_{i^{*}}-2\lambda^{a}_{t_{i+2}+d_{max}+K}
    \]
   Since $\mathcal{F}$ does not occur, $n_{t_{i+2}+d_{max}+K}(i),n_{t_{i+2}+d_{max}+K}({i^*}) \geq (q(\sigma(i))/2) m_{t_{i+2}}(i) = 16\log(T)/\epsilon_{i+2}^{2}$.
    So we get that, 
    \[
        \mu_{i^{*}}-\mu_i=\Delta_i\leq 2\epsilon_{i+2}=\epsilon_{i+1}
    \]
    Contradicting $a \in S_i$. Thus, the total regret from arms in $S_{i}$ is at most
    \begin{align*}
        \sum_{a\in S_{i}}m^{a}_{t_{i+2}+d_{max}+K}\Delta_i & =\sum_{a\in S_{i}}\big(m^{a}_{t_{i+2}+d_{max}+K}-m^{a}_{t_{i+2}}\big)\Delta_i+\sum_{a\in S_{i}}m^{a}_{t_{i+2}}\Delta_i
        \\
         & \leq \epsilon_{i}\sum_{a\in S_{i}}\big(m^{a}_{t_{i+2}+d_{max}+K}-m^{a}_{t_{i+2}}\big)+\sum_{a\in S_{i}}\frac{32\log(T)}{q(i)\epsilon_{i+2}^{2}}\Delta_i
         \\
         & \leq \epsilon_{i}\sum_{a}\big(m^{a}_{t_{i+2}+d_{max}+K}-m^{a}_{t_{i+2}}\big)+\sum_{a\in S_{i}}\frac{512\log(T)}{q(\sigma(i))\Delta_i}
         \\
         & \leq \epsilon_{i}(t_{i+2}-t_{i+2}+d_{max}+K)+\sum_{a\in S_{i}}\frac{512\log(T)}{q(\sigma(i))\Delta_i}
         \\
         & = \epsilon_{i}(d_{max}+K)+\sum_{a\in S_{i}}\frac{512\log(T)}{q(\sigma(i))\Delta_i}
    \end{align*}
    Summing over all $i$ would give us a total regret of 
    \[
    \mathcal{R_{T}\leq}\sum_{a \neq a^*}\frac{512\log(T)}{q(\sigma(i))\Delta_i}+2\max_{a \neq a^*}d^{\max\{a, a^*\}}(q(\sigma(i)))+2K.
    \]
    The above is true for any choice of $\{q(i)\}_{i=1}^{\infty}: q(i) \in (0,1]$. Choosing an optimal $\{q(i)\}_{i=1}^{\infty}$ obtains the statement of the theorem.
\end{proof}

% \subsection{Analysis per Arm}
% \cref{thm:se_reward_indep} and \cref{thm:se_reward_indep_refined} analyze SE regret by fixing a qunatile for all arms or sets of arms with relatively close $\Delta$. The problem with this approach is the inability to set a quantile per arm. This could be disastrous if the delay distributions are very different from one another. Here we expand on the analysis with arm-dependent quantile.
% \begin{theorem}
%     \label{thm:se_reward_indep_arms}
%     For reward-independent delay distributions $\{D^a\}_{a=1}^K$, the expected pseudo-regret of \cref{alg:non-phased-SE} is bounded by
%     \begin{align*}
%         \mathcal{R}_{T} & \leq \min_{q^1,...,q^K} \sum_{i\ne i^{*}}\frac{64\log(T)}{\Delta_i}\left(\frac{1}{q_i}+\frac{1}{q_{i^{*}}}\right)+\max_{\sigma\in S_{K}}\sum_{i\ne i^{*}}\frac{d_i(q_i)}{K-\sigma(i)}\Delta_i+d_{i^*}(q_{i^*})\log(K) + K\log(K),
%     \end{align*}
%     where $S_K$ is the set of all permutations of $[K]$. This is explicitly given as,
%     \begin{align*}
%         \mathcal{R}_{T} & \leq \min_{q^1,...,q^K} \sum_{i\ne i^{*}}\frac{64\log(T)}{\Delta_i}\left(\frac{1}{q_i}+\frac{1}{q_{i^{*}}}\right) + 2\max_{i}d_i(q_i)\log(K)+K\log(K),
%     \end{align*}
% \end{theorem}
